# Supplementary material for: Multiple-Relay Slotted ALOHA: Performance Analysis and Bounds
Source: arXiv:1903.03420 source file (2019-03-08)
Supplement: Supplementary file 1 [file appendix_finiteRlnc.tex]

\section{Analysis of \ac{RLC} with Finite Buffer Size}
\label{app:appendix_finite_rlc}
The achievability of the minimum resources in the downlink via \ac{RLC}, demonstrated in Section~\ref{sec:nc}, comes at the price of observing a very large number of uplink slots, $\numulslot$. In other words, before the relays can apply \ac{RLC} on the received packets, a very long observation window --- virtually infinite --- has to expire. During the observation of the uplink, the relays are required to store in memory the correctly received packet. The consequence is two-folded, on the one hand, the memory required for storing the recovered messages becomes very large and may exceed the relays capabilities; on the other hand, the transmitted messages can have timeouts dictated by higher layers possibly triggering retransmissions even before the packet is forwarded to the \ac{GW}.

Answering the important question on how \ac{RLC} will perform for a finite observation interval, lead us to consider the equivalent case of relays equipped with a finite buffers. We leverage on the derived analytical analysis presented in the following, to evaluate the performance of \ac{RLC} under the finite buffers constraint.

The focus is on a scenario with $2$ relays, i.e. $\nrx=2$, but can also be extended to a more general case. The \ac{GW} collects the incoming packets forwarded by the relays building the system of linear equations
\begin{gather}
\left( \begin{array}{c} \colVecK{\{1\}}^T\\ \colVecK{\{2\}}^T \end{array} \right) =
\MxCombRed \linCombRed^T = \\
\left(\begin{array}{ccc} \MxCombRedK{1,\{1\}} & \bm 0 &  \MxCombRedK{1,\{1,2\}} \\
\bm 0 & \MxCombRedK{2,\{2\}} & \MxCombRedK{2,\{1,2\}}
\end{array}\right)
\left( \begin{array}{l} \linCombRedK{\{1\}}^T\\
\linCombRedK{\{2\}}^T \\
\linCombRedK{\{1,2\}}^T
\end{array} \right),
\label{eq:exampleG_K=2}
\end{gather}
with $\MxCombRedK{1,\{1\}} \in \mathbb{F}_{2^L}^{\rpkK{1} \times \collK{1}}$ being the matrix representing the coefficients applied to linear combinations of uplink decoded packets by the first relay only. Likewise, $\MxCombRedK{2,\{2\}} \in \mathbb{F}_{2^L}^{\rpkK{2} \times \collK{2}}$ is the matrix representing the coefficients applied to linear combinations of uplink decoded packets by the second relay only. Finally, $\MxCombRedK{1,\{1,2\}} \in \mathbb{F}_{2^L}^{\rpkK{1} \times \collK{1,2}}$ and $\MxCombRedK{2,\{1,2\}} \in \mathbb{F}_{2^L}^{\rpkK{2} \times \collK{1,2}}$ are the coefficients of the packets linear combinations generated respectively by the first and second relay involving uplink decoded packets by both relays. The vector $\linCombRed$ corresponds to the uplink decoded packets, where $\linCombRedK{\{1\}}$, $\linCombRedK{\{2\}}$ are the uplink decoded packets by the first and second relay respectively, and $\linCombRedK{\{1,2\}}$ are the uplink decoded packets by both of them. The vectors $\colVecK{\{1\}}$ and $\colVecK{\{2\}}$ represent the linear combinations of packets received at the \ac{GW} generated by the first and second relay respectively.

\begin{sloppypar}
The GW applies Gauss-Jordan elimination, in order to solve the system of equations. After some operations including columns and rows reordering it obtains $\MxCombRed'$ as
\begin{align}
\MxCombRed' =
\left( \begin{array}{ccc|ccc}
\bm{I}_{\rankK{1}} & \bm{0} & \bm{0} & \bm{A} & \bm{0} & \bm{U}_1 \\
\bm{0} & \bm{I}_{\rankK{2}} & \bm{0} & \bm{0} & \bm{B} & \bm{U}_2 \\
\bm{0} & \bm{0} & \bm{I}_{\rankK{1,2}} & \bm{0} & \bm{0} & \bm{L} \\
\hline
\bm{0} & \bm{0} & \bm{0} & \bm{0} & \bm{0} & \bm{0}
\end{array}
\right).
\label{eq:Mx_second_two}
\end{align}
Where the identity matrix with size $x$ is denoted with $\bm{I}_x$. The sizes $\rankK{1}$ and $\rankK{2}$ represent the rank of the matrices $\MxCombRedK{1,\{1\}}$ and $\MxCombRedK{2,\{2\}}$ respectively. The matrices $\bm{A} \in \mathbb{F}_{2^L}^{\rankK{1}\times \mxColK{1}}$ and $\bm B \in \mathbb{F}_{2^L}^{\rankK{2} \times \mxColK{2}}$ collect all non-zero elements left after Gauss-Jordan elimination on matrices $\MxCombRedK{1,\{1\}}$ and $\MxCombRedK{2,\{2\}}$. For ease of notation we denote $\mxColK{1}=\collK{1}-\rankK{1}$ and $\mxColK{2}=\collK{2}-\rankK{2}$. The matrices $\bm{U}_1 \in \mathbb{F}_{2^L}^{\rankK{1} \times \mxColK{1,2}}$, $\bm{U}_2 \in \mathbb{F}_{2^L}^{\rankK{2} \times \mxColK{1,2}}$ and $\bm{L} \in \mathbb{F}_{2^L}^{\rankK{1,2} \times \mxColK{1,2}}$, where $\rankK{1,2}\leq \left[(\rpkK{1} + \rpkK{2}) - (\rankK{1} + \rankK{2})\right]$ and $\mxColK{1,2}=\collK{1,2}-\rankK{1,2}$.

The downlink throughput is defined as the average number of correctly collected packets per uplink timeslot, or
\begin{equation}
\label{eq:th_dw}
\tpDL = \frac{\mathbb{E}[\collRV]}{\numulslot} = \frac{\mathbb{E}[C_1] + \mathbb{E}[C_2] + \mathbb{E}[C_{1,2}]}{\numulslot}.
\end{equation}
The expectation is split into the average number of collected packets forwarded only by the first relay to the gateway, $\mathbb{E}[C_1]$. Likewise, $\mathbb{E}[C_2]$ is the average number of collected packets forwarded only by the second relay to the gateway, and the average number of collected packets forwarded by both relays to the gateway is $\mathbb{E}[C_{1,2}]$. We first elaborate on $\mathbb{E}[C_1]$, and exploiting the chain rule of probability, we can write
\begin{equation}
\begin{aligned}
\label{eq:exp_c1}
\mathbb{E}[C_1] &= \sum_{\substack{\collK{1},\collK{2},\\ \collK{1,2}}} \sum_{\substack{\rankK{1},\rankK{2},\\ \rankK{1,2}}} \mathbb{E}[C_1|\collK{1},\collK{2},\collK{1,2}, \rankK{1},\rankK{2},\rankK{1,2}] \\
&\cdot \Pr(\rankK{1}|\collK{1}) \Pr(\rankK{2}|\collK{2})\Pr(\rankK{1,2}|\collK{1,2},\rankK{1},\rankK{2})\\
&\cdot \Pr(\collK{1},\collK{2},\collK{1,2}).
\end{aligned}
\end{equation}
To successfully decode a specific packet at the \ac{GW}, we require that its corresponding row in the matrix $\MxCombRed'$ has only one non-zero element. This event has probability $\left(\frac{1}{2^L}\right)^{\mxColK{1}+\mxColK{3}}$. Consequently, $\mathbb{E}[C_1|\collK{1},\collK{2},\collK{1,2}, \rankK{1},\rankK{2},\rankK{1,2}]$ is the mean of the binomial distribution $\mathcal{B}\left(\collK{1}, \frac{1}{\left(2^L\right)}^{\mxColK{1}+\mxColK{3}}\right)$, and it holds
\begin{equation}
\mathbb{E}[C_1|\collK{1},\collK{2},\collK{1,2}, \rankK{1},\rankK{2},\rankK{1,2}] = \collK{1} \left(\frac{1}{2^L}\right)^{\mxColK{1}+\mxColK{3}}
\end{equation}
%Now, we can write
%\begin{align}
%\mathbb{E}[\widehat N_1] &= \sum_{\colNumVec} \sum_{\rankNumVec} \collK{1}\left( \frac{1}{\fieldOrd}\right)^{\mxColK{1}+ \mxColK{3}} \Pr(\rankNumVec| \colNumVec) \Pr(\colNumVec) =\\
%&= \sum_{\collK{1}=0}^{\numulslot} \sum_{\collK{2}=0}^{\numulslot} \sum_{\collK{1\wedge2}=0}^{\numulslot} \sum_{\rankK{1}=0}^{\rankKMax{1}} \sum_{\rankK{2}=0}^{\rankKMax{2}} \sum_{\rankK{3}=0}^{\rankKMax{3}} \collK{1}\left( \frac{1}{\fieldOrd}\right)^{\mxColK{1}+\mxColK{3}} \\
%&\cdot \Pr(\rankK{1}|\collK{1}) \Pr(\rankK{2}|\collK{2})  \Pr(\rankK{3}|\collK{1\wedge2}) \\
%&\cdot \Pr(\collK{1},\collK{2},\collK{1\wedge2}),
%\label{eq:n1_avg}
%\end{align}
%where $\rankKMax{1}=\min \{\linllK{1},\collK{1}\}$, $\rankKMax{2}=\min \{\linllK{2},\collK{2}\}$ and $\rankKMax{3}=\min \{(\linllK{1} + \linllK{2}) - (\rankK{1} + \rankK{2}), \collK{1\wedge2}\}$. The last equality holds because the rank of the sub-matrices $\rankK{1}$, $\rankK{2}$ and $\rankK{3}$ are independent with each other. The Markov chains that show how the rank of the matrix evolves as row vectors $\mathbb{F}_{\fieldOrd}^{1 \times \coll}$ are added one by one as shown in Figure~\ref{fig:Mk_chain_rank}. The probability that a matrix belonging to $\mathbb{F}_{\fieldOrd}^{\rank \times \coll}$ has rank $x_{\rank}= \min\{\rank,\coll\}$ can be written in a recursive way \cite{Landsberg_1893, Kolchin_RG_1999} as

The probability that a generic matrix with elements in $\mathbb{F}_{2^L}$ has rank $\rankK{1}$ given that is constituted by $\rpkK{1}$ rows and $\collK{1}$ columns, can be recursively computed. Pursuing this aim, we first compute the probability that the prototype matrix composed by one row and $\collK{1}$ columns, has rank $\rankK{1} = 0,1$, i.e.%
\begin{equation}
\begin{aligned}
\Prob_{1,\collK{1}}(0) &= \left(\frac{1}{2^L}\right)^{\collK{1}}\\
\Prob_{1,\collK{1}}(1) &= 1-\left(\frac{1}{2^L}\right)^{\collK{1}}.%
\end{aligned}%
\end{equation}%
\end{sloppypar}%
The generic recursion follows as
\begin{equation}
\label{eq:mx_recursion}
\begin{aligned}
\Pr(\rankK{1}|\collK{1}) &=\Prob_{\rpkK{1},\collK{1}}(\rankK{1}) =\left(2^L\right)^{(\rankK{1}-\collK{1})}\Prob_{\rpkK{1}-1,\collK{1}}(\rankK{1})\\
&+ \left(1-\left(2^L\right)^{(\rankK{1}-\collK{1}-1)}\right) \Prob_{\rpkK{1}-1,\collK{1}}(\rankK{1}-1)\\
& \qquad \qquad \text{with $\rankK{1}=0,1,...,\min\{\rpkK{1},\collK{1}\}$.}
\end{aligned}
\end{equation}
The results can be straightforwardly applied also to the second probability $\Pr(\rankK{2}|\collK{2})$. Similarly, for computing $\Pr(\rankK{1,2}|\collK{1,2},\rankK{1},\rankK{2})$ we denote with $\bar{\rpk}=\rpkK{1}+\rpkK{2}-(\rankK{1}+\rankK{2})$, the number of rows in the matrix. Substituting the proper matrix dimension in equation \eqref{eq:mx_recursion}, we obtain this probability. The joint probability mass function $\Pr(\collK{1},\collK{2}, \collK{1,2})$ can be tracked effectively by means of a homogeneous Markov chain, leaning on the assumed independence of channel realizations across uplink slots. To this aim, let $\obsSlot_\slot = \colVecNum = \{ \collK{1}, \collK{2}, \collK{1,2} \}$ be the state at the start of slot $\slot$, indicating the number of packets received so far by the first relay solely, by the second relay and by both of them, respectively. For the sake of compactness, let us furthermore denote $\textrm{Pr}\left\{ \obsSlot_{\slot+1}\, \big{|} \, \obsSlot_\slot \right\}$ as $\Prob_{\colVecNum,\colVecNum'}$. Following this notation, each time unit can see five possible transitions for the chain, whose probabilities follow by simple combinatorial arguments similar to the ones discussed in Section~\ref{sec:uplink}:

%To this aim, let $\obsSlot_\slot = \{ \collK{1}^{(\slot)}, \collK{2}^{(\slot)}, \collK{1,2}^{(\slot)} \}$ be the state at the start of slot $\slot$, indicating the number of packets received so far by the first relay solely, by the second relay and by both of them, respectively. For the sake of compactness, let us furthermore denote $\textrm{Pr}\left\{ \obsSlot_{\slot+1} = \{ i',j',k'\}  \, \big{|} \, \obsSlot_\slot = \{ i,j,k  \} \right\}$ as $\Prob_{(i,j,k)\rightarrow(i',j',k')}$. Following this notation, each time unit can see five possible transitions for the chain, whose probabilities follow by simple combinatorial arguments similar to the ones discussed in Section~\ref{sec:uplink}:
%\begin{equation}
%\begin{cases}
%\begin{aligned}
%\Prob_{(i,j,k)\rightarrow(i,j,k)}
%&= 1 - 2\load (1-\peras) e^{-\load (1-\peras)}\\ &+ \load ( 1-\peras )^2\, e^{-\load (1-\peras^2)} \left( 1+\load \peras^2\right) \\
%\Prob_{(i,j,k)\rightarrow(i+1,j,k)}
%&= \load (1-\peras) e^{-\load (1-\peras)}\\ &- \load ( 1-\peras )^2\, e^{-\load (1-\peras^2)} \left( 1+\load \peras^2\right) \\
%\Prob_{(i,j,k)\rightarrow(i,j+1,k)}
%&= \load (1-\peras) e^{-\load (1-\peras)}\\ &- \load ( 1-\peras )^2\, e^{-\load (1-\peras^2)} \left( 1+\load \peras^2\right) \\
%\Prob_{(i,j,k)\rightarrow(i,j,k+1)}
%&= \load ( 1-\peras )^2\, e^{-\load (1-\peras^2)} \\
%\Prob_{(i,j,k)\rightarrow(i+1,j+1,k)}
%&=  (\load \peras)^2\,( 1-\peras )^2\, e^{-\load (1-\peras^2)} \\
%\end{aligned}
%\end{cases}
%\label{eq:markov_transitions}
%\end{equation}

\begin{sloppypar}
\begin{equation}
\begin{aligned}
\Prob_{\colVecNum,\colVecNum} &= 1 - \tpULk{2} \\
\Prob_{\colVecNum,\colVecNum+\bm{e}_1} &= \tpULk{2} - ( \tpSA + \tpX ) \\
\Prob_{\colVecNum,\colVecNum+\bm{e}_2} &= \tpULk{2} - ( \tpSA + \tpX ) \\
\Prob_{\colVecNum,\colVecNum+\bm{e}_3} &= 2\,\tpSA - \tpULk{2} \\
\Prob_{\colVecNum,\colVecNum+\bm{e}_1+\bm{e}_2} &=  \tpX \\
\end{aligned}
\label{eq:markov_transitions}
\end{equation}
We recall that ${\tpSA = \load (1-\peras) e^{-\load(1-\peras)}}$, ${\tpULk{2} = 2\load (1-\peras)\, e^{-\load (1-\peras)} - \load (1-\peras)^2 \, e^{-\load (1-\peras^2)}}$. We denote with ${\tpX = (\load \peras)^2 (1-\peras)^2 \, e^{-\load (1-\peras^2)}}$ and the three standard basis vectors of the three dimensional space as $\bm{e}_1=\{1,0,0\}$, $\bm{e}_2=\{0,1,0\}$ and $\bm{e}_3=\{0,0,1\}$. The defined probabilities uniquely identify the transition matrix for the Markov chain under consideration, so that the sought probability mass function follows as its $\numulslot$-th step evolution when forcing the initial state as $\obsSlot_0 = \{0,0,0\}$.
\end{sloppypar}
In order to finalize the computation of the donwlink throughput of equation \eqref{eq:th_dw}, we still need to compute $\mathbb{E}[C_2]$ and $\mathbb{E}[C_{1,2}]$. Fortunately, these quantities differ from the expression of $\mathbb{E}[C_1]$ of equation \eqref{eq:exp_c1}, only in the first addend, which can be easily computed as,
\begin{equation}
\mathbb{E}[C_2|\collK{1},\collK{2},\collK{1,2}, \rankK{1},\rankK{2},\rankK{1,2}] = \collK{2} \left(\frac{1}{2^L}\right)^{\mxColK{2}+\mxColK{3}}
\end{equation}
\begin{equation}
\mathbb{E}[C_{1,2}|\collK{1},\collK{2},\collK{1,2}, \rankK{1},\rankK{2},\rankK{1,2}] = \collK{1,2} \left(\frac{1}{2^L}\right)^{\mxColK{3}}.
\end{equation}
